# Supplementary material for: Federated Model Distillation with Noise-Free Differential Privacy
Source: arXiv:2009.05537 source file (2021-05-21)
Supplement: Supplementary file 1 [file appendix.tex]

\begin{table*}[h]
  \caption{Models for MNIST/FEMNIST}
  \label{model-MNIST}
  \centering
\begin{tabular}{ |p{1.5cm}||p{2cm}|p{2cm}|p{2cm}|p{1.5cm}|p{2cm}| }
 \hline
% \multicolumn{4}{|c|}{Country List} \\
Local model & 1st conv layer filters ($n_1$)& 2nd conv layer filters ($n_2)$ & 3 conv layer filters ($n_3$) & dropout rate&pre-trained test accuracies on MNIST\\ 
 \hline\hline
0 & 128 & 256 &  None & 0.2&98.6\%\\
1 & 128 & 384 &  None & 0.2&98.8\%\\
2 & 128 & 512 &  None & 0.2&98.4\%\\
3 & 256 & 256 &  None & 0.3 &98.3\%\\
4 & 256 & 512 &  None & 0.4&98.2 \%\\
5 & 64 & 128 &  256 & 0.2&98.9\%\\
6 & 64 & 128 &  192 & 0.2 &99.0\%\\
7 & 128 & 192 &  256 &0.2 &99.1\%\\
8 & 128 & 128 &  128 &0.3&99.2\%\\
9 & 128 & 128 &  192 &0.3&98.9\%\\
 \hline
\end{tabular}
\label{table:models_MNIST}
\end{table*}

\begin{table*}[h]
  \caption{Models for CIFAR10/CIFAR100}
  \label{model-CIFAR10}
  \centering
\begin{tabular}{ |p{1cm}||p{2cm}|p{2cm}|p{2cm}|p{2cm}|p{1.3cm}|p{2cm}|}
 \hline
% \multicolumn{4}{|c|}{Country List} \\
Local model & 1st conv layer filters ($n_1$)& 2nd conv layer filters ($n_2$) & 3rd conv layer filters ($n_3$) 
& 4th conv layer filters ($n_4$) & dropout rate & pre-trained test accuracies on CIFAR10\\ 
 \hline\hline
0 & 128 & 256 &  None & None& 0.2&  71.5\%\\
1 & 128 & 128 &  192 & None & 0.2&  78.8\%\\
2 & 64 & 64 &  64 & None & 0.2&  75.5\%\\
3 & 128 & 64 &  64 & None & 0.3&  74.5\%\\
4 & 64 & 64 & 128 & None & 0.4& 74.9\%\\
5 & 64 & 128 &  256 & None &  0.2 &  74.8\%\\
6 & 64 & 128 &  192 & None & 0.2 &  77.5\%\\
7 & 128 & 192 &  256 & None &0.2 & 77.7\%\\
8 & 128 & 128 &  128 & None & 0.3& 78.8\%\\
9 & 64 & 64 & 64 & 64 & 0.2& 75.4\%\\
 \hline
\end{tabular}
\label{table:models_CIFAR}
\end{table*}
